# Supplementary material for: Reservoir Computing with Diverse Timescales for Prediction of Multiscale Dynamics
Source: arXiv:2108.09446 source file (2022-07-29)
Supplement: Supplementary file 1 [file supplemental.pdf]

# Supplemental material:
# Reservoir computing with diverse timescales for prediction of multiscale dynamics

Gouhei Tanaka[1,2,3,*], Tadayoshi Matsumori[4], Hiroaki Yoshida[4], and Kazuyuki Aihara[1]
[1] *International Research Center for Neurointelligence, The University of Tokyo, Tokyo 113-0033, Japan*
[2] *Department of Electrical Engineering and Information Systems, Graduate School of Engineering, The University of Tokyo, Tokyo 113-8656, Japan.*
[3] *Department of Mathematical Informatics, Graduate School of Information Science and Technology, The University of Tokyo, Tokyo 113-8656, Japan.*
[4] *Toyota Central Research and Development Laboratory Inc. Tokyo, Japan.*

## I. DERIVATION OF THE DTS-ESN

The continuous-time system corresponding to the update of reservoir states in the diverse-timescale ESN (DTS-ESN: Eq. (1) in the main text) is described as follows:

$$c_i \frac{\mathrm{d}x_i(t)}{\mathrm{d}t} = -x_i(t) + f(h_i(t)) \quad \text{for } i = 1, \dots, N_x, \tag{S1}$$

where $x_i(t)$ is the $i$-th component of the reservoir state vector $\mathbf{x}(t)$, $h_i(t)$ is the $i$-th component of the internal state vector $\mathbf{h}(t) = \rho W \mathbf{x}(t) + \gamma W^{\mathrm{in}} \mathbf{u}(t) + \zeta W^{\mathrm{fb}} \mathbf{y}(t)$, and $c_i$ is the coefficient scaling the time constant for neuron $i$ in the reservoir. The DTS-ESN is derived by discretizing the above model in time using the Euler method in a similar way to the derivation of the LI-ESN [1]. By applying the Euler discretization with time step $\Delta t$, i.e.

$$\frac{\mathrm{d}x_i(t)}{\mathrm{d}t} \approx \frac{x_i(t+\Delta t) - x_i(t)}{\Delta t}, \tag{S2}$$

we can rewrite Eq. (S1) as follows:

$$x_i(t+\Delta t) = \left(1 - \frac{\Delta t}{c_i}\right) x_i(t) + \frac{\Delta t}{c_i} f(h_i(t)) \quad \text{for } i = 1, \dots, N_x. \tag{S3}$$

By defining the leak rate as $\alpha_i \equiv \Delta t / c_i$, we obtain the following equation:

$$x_i(t+\Delta t) = (1 - \alpha_i)\, x_i(t) + \alpha_i f(h_i(t)) \quad \text{for } i = 1, \dots, N_x. \tag{S4}$$

This is equivalent to Eq. (1) in the main text, described as follows:

$$\mathbf{x}(t+\Delta t) = (I - A)\mathbf{x}(t) + A f(\mathbf{h}(t)), \tag{S5}$$

where $A = \mathrm{diag}(\alpha_1, \dots, \alpha_{N_x})$.

## II. TIMESCALES AND EIGENVALUES

### II-A. Timescales of linearized systems

The time evolution of the reservoir state in the DTS-ESN is described as Eq. (S5). By linearizing Eq. (S5) at the fixed point at the origin, we obtain a linearized dynamical system as follows:

$$\mathbf{x}(t+\Delta t) = J \mathbf{x}(t), \tag{S6}$$

where $J$ is the Jacobian matrix. Note that the linearized system of the LI-ESN can also be described in the above form. Assuming that $J$ is diagonalizable, we have the following equation:

$$P^{-1} J P = \Lambda, \tag{S7}$$

where $\Lambda = \mathrm{diag}(\lambda_1, \dots, \lambda_{N_x})$ is a diagonal matrix composed of the eigenvalues of $J$, and $P$ is a matrix composed of the corresponding eigenvectors. By using a variable transformation $\mathbf{y}(t) = P^{-1}\mathbf{x}(t)$, we can rewrite Eq. (S6) as follows:

$$\mathbf{y}(t+\Delta t) = \Lambda \mathbf{y}(t), \tag{S8}$$

which is a set of independent $N_x$ linear difference equations. The solution of the $i$-th equation is given by

$$\begin{aligned} y_i(t) &= \lambda_i^{t/\Delta t} y_i(0) \\ &= |\lambda_i|^{t/\Delta t}(\cos((t/\Delta t)\theta_i) + j\sin((t/\Delta t)\theta_i))y_i(0), \end{aligned} \tag{S9}$$

where $j$ denotes the imaginary unit, $\mathrm{Re}(\lambda_i) = |\lambda_i|\cos\theta_i$, and $\mathrm{Im}(\lambda_i) = |\lambda_i|\sin\theta_i$. Since $|\lambda_i|^{t/\Delta t} = e^{(t/\Delta t)\ln|\lambda_i|}$, the exponential decay rate with regard to neuron $i$ in the reservoir is expressed as follows:

$$t/\tau_i = -(t/\Delta t)\ln|\lambda_i|, \tag{S10}$$

where $\tau_i$ is the timescale of the dynamics of neuron $i$ in the reservoir. Hence we have Eq. (5) in the main text:

$$\tau_i = -\frac{\Delta t}{\ln|\lambda_i|}. \tag{S11}$$

### II-B. Difference between DTS-ESN and LI-ESN

The distribution of timescales realized by the DTS-ESN is largely different from that by the LI-ESN (see Figure 2 in the main text). Here we observe their difference in terms of the eigenvalue distribution of the Jacobian matrix.

The Jacobian matrix of the linearized system of the LI-ESN is given by

$$J_{\mathrm{L}} = I - \alpha I + \rho\alpha W, \tag{S12}$$

where $\alpha$ is the leak rate common to all the reservoir neurons, $W$ is the recurrent weight matrix of the reservoir, and $\rho$ is the spectral radius of $\rho W$. Since $W$ is scaled so that its spectral radius (i.e. the maximum absolute eigenvalue) is unity, the eigenvalues of $W$, denoted by $\lambda_i^{(W)}$ ($i = 1, \ldots, N_x$), are uniformly distributed over the unit disk on the complex plane. The eigenvalues of $J_{\mathrm{L}}$, denoted by $\lambda_i^{(J_{\mathrm{L}})}$, can be described as follows [2]:

$$\lambda_i^{(J_{\mathrm{L}})} = 1 - \alpha + \rho\alpha\lambda_i^{(W)} \quad \text{for } i = 1, \ldots, N_x. \tag{S13}$$

The distribution of these eigenvalues for different $\alpha$ values are shown in Fig. S1(a). The eigenvalue distribution is a circular uniform distribution over a circle with radius $\rho\alpha$, centered at $1 - \alpha$. When $\rho = 1$, the original circular distribution at $\alpha = 1$ (solid curve) drastically shrinks with a decrease in the $\alpha$ value, and eventually all the eigenvalues converge to 1 on the real axis in the limit of $\alpha \to 0$. The leak rate $\alpha$ has a role to restrict the range of timescales as shown in Fig. 2 in the main text, because both the maximum and minimum values of $-1/\ln|\lambda_i^{(J_{\mathrm{L}})}|$ (see Eq. (S11)) monotonically increases as $\alpha$ is decreased.

On the other hand, the Jacobian matrix of the linearized system of the DTS-ESN is given by

$$J_{\mathrm{D}} = I - A + \rho A W, \tag{S14}$$

where $A = \mathrm{diag}(\alpha_1, \ldots, \alpha_{N_x})$ is the diagonal matrix of leak rates of the neurons in the reservoir. The $(i,j)$ entry of $J_{\mathrm{D}}$ is given by $1 - \alpha_i + \rho\alpha_i w_{ij}$. Since both $\alpha_i$ and $w_{ij}$ are randomly generated, $J_{\mathrm{D}}$ can be viewed as a random matrix. The distribution of the eigenvalues of $J_{\mathrm{D}}$, denoted by $\lambda_i^{(J_{\mathrm{D}})}$, is shown in Fig. S1(b). When $\alpha_{\min}$ is decreased from 1,

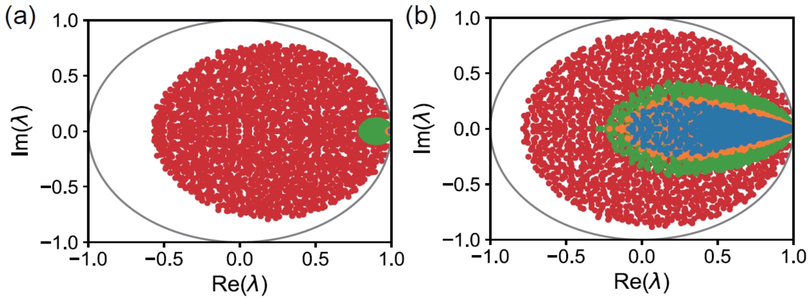


FIG. S1. Distributions of eigenvalues of the Jacobian matrices. The parameter values were set at $N_x = 2000$, $d = 0.1$, $\rho = 1$, and $\Delta t = 1$. (a) The LI-ESN. The leak rate $\alpha$ was set at $10^{-0.1}$ (red), $10^{-1}$ (green), $10^{-2}$ (orange), and $10^{-3}$ (blue). (b) The DTS-ESN with $\alpha_{\max} = 1$. The value of $\alpha_{\min}$ was set at $10^{-0.1}$ (red), $10^{-1}$ (green), $10^{-2}$ (orange), and $10^{-3}$ (blue).

the range of the eigenvalue distribution shrinks and the maximum value of $-1/\ln|\lambda_i^{(J_\mathrm{D})}|$ monotonically increases. We notice that the eigenvalues close to the origin (i.e. those with small $|\lambda_i^{(J_\mathrm{D})}|$) remain owing to the random distribution of $\alpha_i$. As a result, the diverse timescales can be realized in the DTS-ESN (see Fig. 2 in the main text).

If the eigenvalue distribution of $J_\mathrm{D}$ is analytically derived, the probabilistic distribution function of the timescales in the DTS-ESN could be obtained. We have explored this possibility based on the random matrix theory, but it is still under investigation.

## III. ONE-STEP-AHEAD PREDICTION (TASK 1)

### III-A. Examples of predictions by the DTS-ESN

Figure S2 demonstrates examples of predicted time series by the DTS-ESN in the one-step-ahead prediction task (Task 1). Figure S2(a) shows the histogram of leak rates $\alpha_i$ generated from a log-uniform distribution in $[10^{-3}, 1]$. Figure S2(b)-(e) show the predictions of the DTS-ESN (red: fast, blue: slow) for the Rulkov, HR, tc-VdP, and tc-Lorenz systems, respectively, which are superimposed on the target dynamics (black). We can see that the slow dynamics is well predicted using only the input time series generated from the fast subsystem.

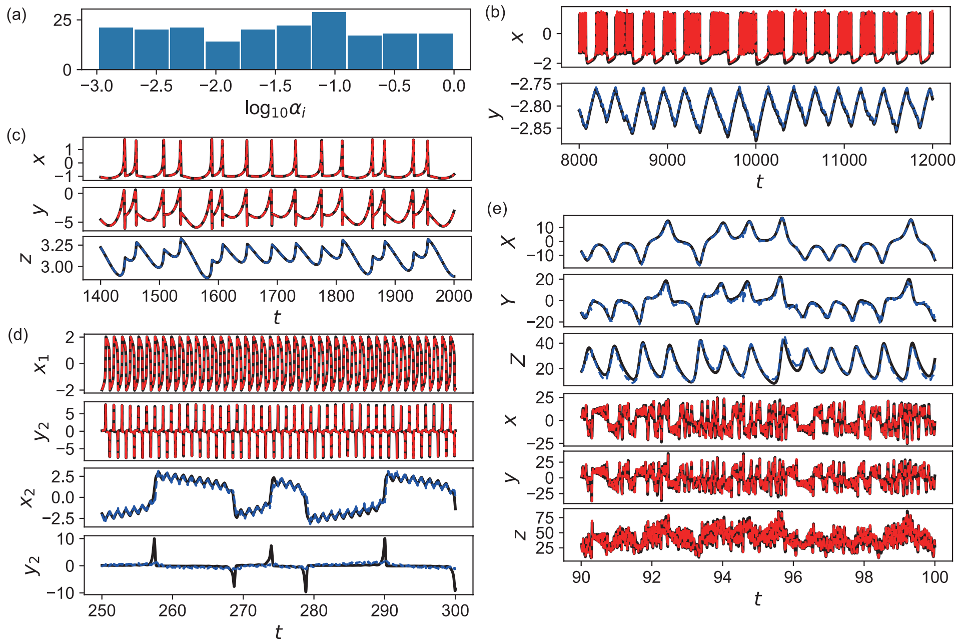

FIG. S2. Examples of predictions by the DTS-ESN. The predicted time series are indicated by colored lines (red: fast, blue: slow). The target time series are indicated by black lines. The parameter values are the same as those for Fig. 3 in the main text but with $\alpha_{\min} = 10^{-3}$. (a) The histogram of $\log_{10}\alpha_i$ in $[10^{-3}, 1]$. (b) The Rulkov model. (c) The Hindmarsh-Rose model. (d) The tc-VdP model. (e) The tc-Lorenz model.

### III-B. Hyperparameter dependence

Figure 3 in the main text shows the NRMSEs with respect to all the variables in the one-step-ahead prediction task (Task 1). Figure S3 shows the details of the NRMSEs for each variable (red: fast, blue: slow, green: all). The panels with label 'All' correspond to Fig. 3 in the main text. Since the timescale is different depending on the variable (or the component system), the optimal value of $\alpha$ of the LI-ESN, achieving the minimum NRMSE, is different between the variables. This gap in the appropriate $\alpha$ values among the variables makes it difficult to hold down the total prediction error in the LI-ESN. In contrast, the diverse timescales realized by the distributed $\alpha_i$ of the DTS-ESN can accommodate different timescales in the component systems of the target dynamics. As a result, the DTS-ESN with highly distributed leak rates is favorable for achieving small prediction errors.

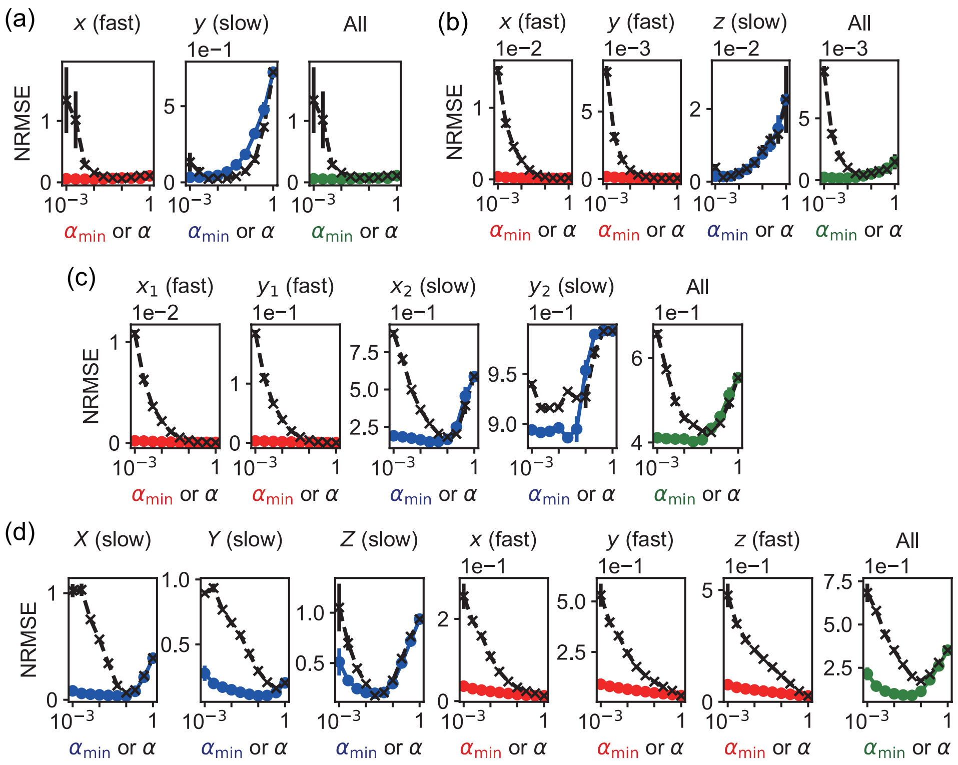


FIG. S3. Comparisons of NRMSEs between the DTS-ESN (colored circles) and the LI-ESN (black crosses) in Task 1. The horizontal axis is $\alpha_{\min}$ for the DTS-ESN and $\alpha$ for the LI-ESN. The red, blue, and green colors correspond to the fast, slow, and whole variables, respectively. The hyperparameter and data settings are the same as those for Fig. 3 of the main text. (a) The Rulkov model. (b) The Hindmarsh-Rose model. (c) The tc-VdP model. (d) The tc-Lorenz model.

In Fig. 3 of the main text, we fixed the hyperparameter values other than the leak rates. To validate the benefit of the DTS-ESN, we examined the influence of some hyperparameter values and data length. In the first case, we doubled the number of the reservoir neurons, $N_x$. In the second case, we doubled the length of the training period, $T_{\mathrm{train}}$. In the third case, we doubled both $N_x$ and $T_{\mathrm{train}}$. The other hyperparameter values are the same as those used for Fig. 3 of the main text. The results are shown in Fig. S4. We can confirm that the comparative results for the DTS-ESN and the LI-ESN are qualitatively the same as those in Fig. 3 of the main text. From a comparison among the three cases for each target system, we can see that the doubling of the reservoir size and the training period reduce the prediction error. For instance, the NRMSE of the DTS-ESN at $\alpha_{\min} = 10^{-3}$ for the tc-Lorenz model is obviously decreased as shown in Fig. S4(c). This suggests that the advantage of the DTS-ESN over the LI-ESN is more enhanced with a larger-size reservoir and a larger number of training data.

We also examined the effects of the input scaling factor $\gamma$ and the spectral radius $\rho$ (in addition to the leak rates) on the predictive performance. Figure S5 shows the dependence of the NRMSE on $\gamma$ (vertical axis) when $\alpha_{\min}$ is varied for the DTS-ESN (upper panels) and $\alpha$ is varied for the LI-ESN (lower panels). A darker color corresponds to a smaller error. From the comparison between the upper and lower panels for each variable of each target system, we can see that the DTS-ESN has more darker parameter regions compared to the LI-ESN. In a similar way, Fig. S6 shows the dependence of the NRMSE on $\rho$ (vertical axis). As in the previous figure, the DTS-ESN is better than the LI-ESN in the large parameter regions.

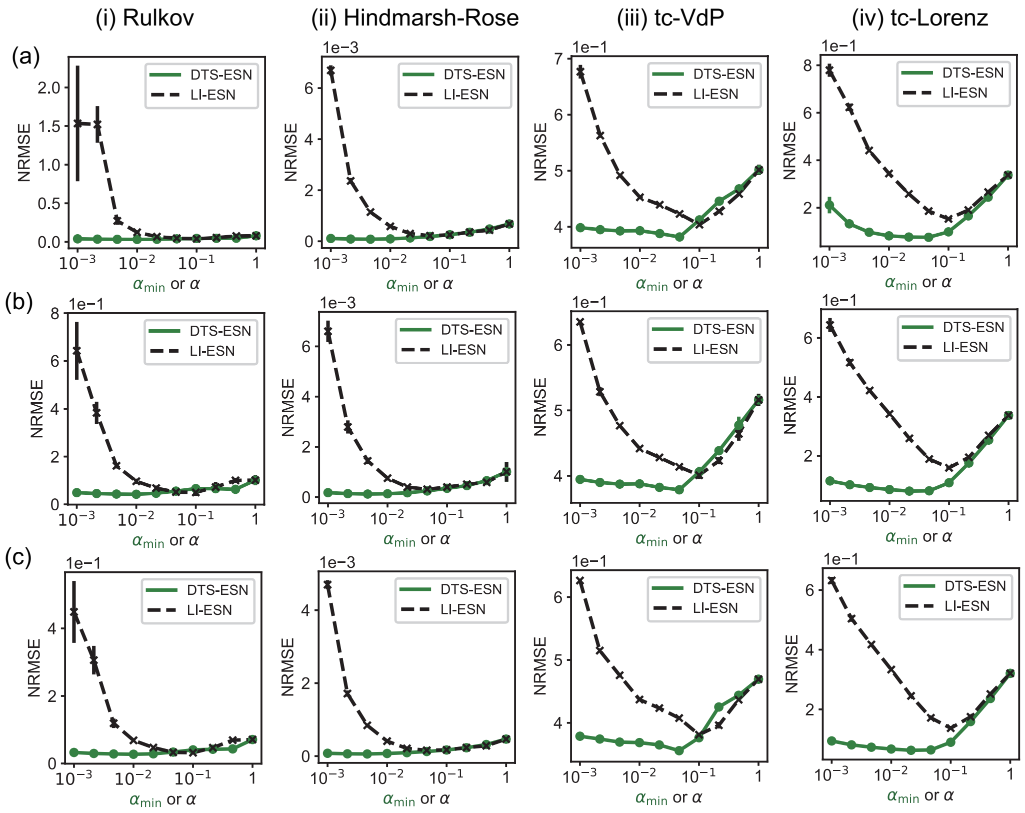


FIG. S4. Comparisons of the NRMSE between the DTS-ESN (green circles) and the LI-ESN (black crosses) in the one-step-ahead prediction task (Task 1). The hyperparameter and data settings are the same as those for Fig. 3 in the main text except for the modification described as follows. (a) The first case where the number of reservoir size $N_x$ is doubled. (b) The second case where the length of the training period $T_{\mathrm{train}}$ is doubled. (c) The third case where both (a) and (b) were applied.

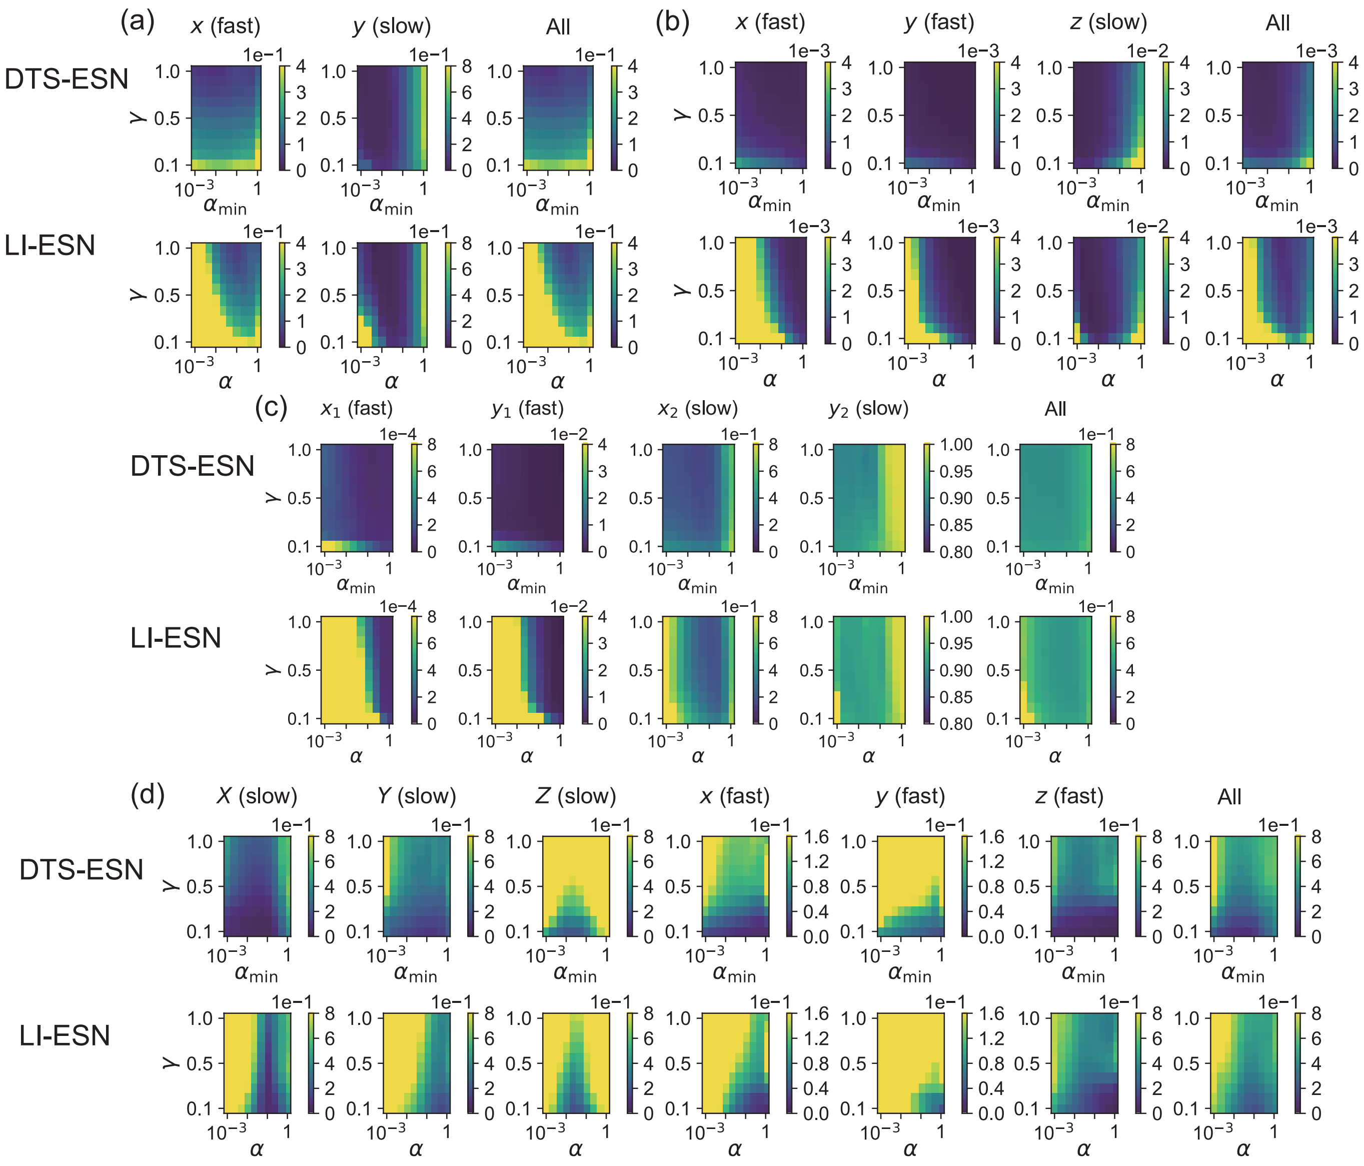


FIG. S5. The effect of the input scaling factor $\gamma$ on the prediction performance of the DTS-ESN (upper panels) and the LI-ESN (lower panels) in Task 1. The color bar indicates the NRMSE. The horizontal axis is $\alpha_{\min}$ for the DTS-ESN and $\alpha$ for the LI-ESN. The hyperparameter and data settings are the same as those for Fig. 3 of the main text, except for the varied ones. (a) The Rulkov model. (b) The Hindmarsh-Rose model. (c) The tc-VdP model. (d) The tc-Lorenz model.

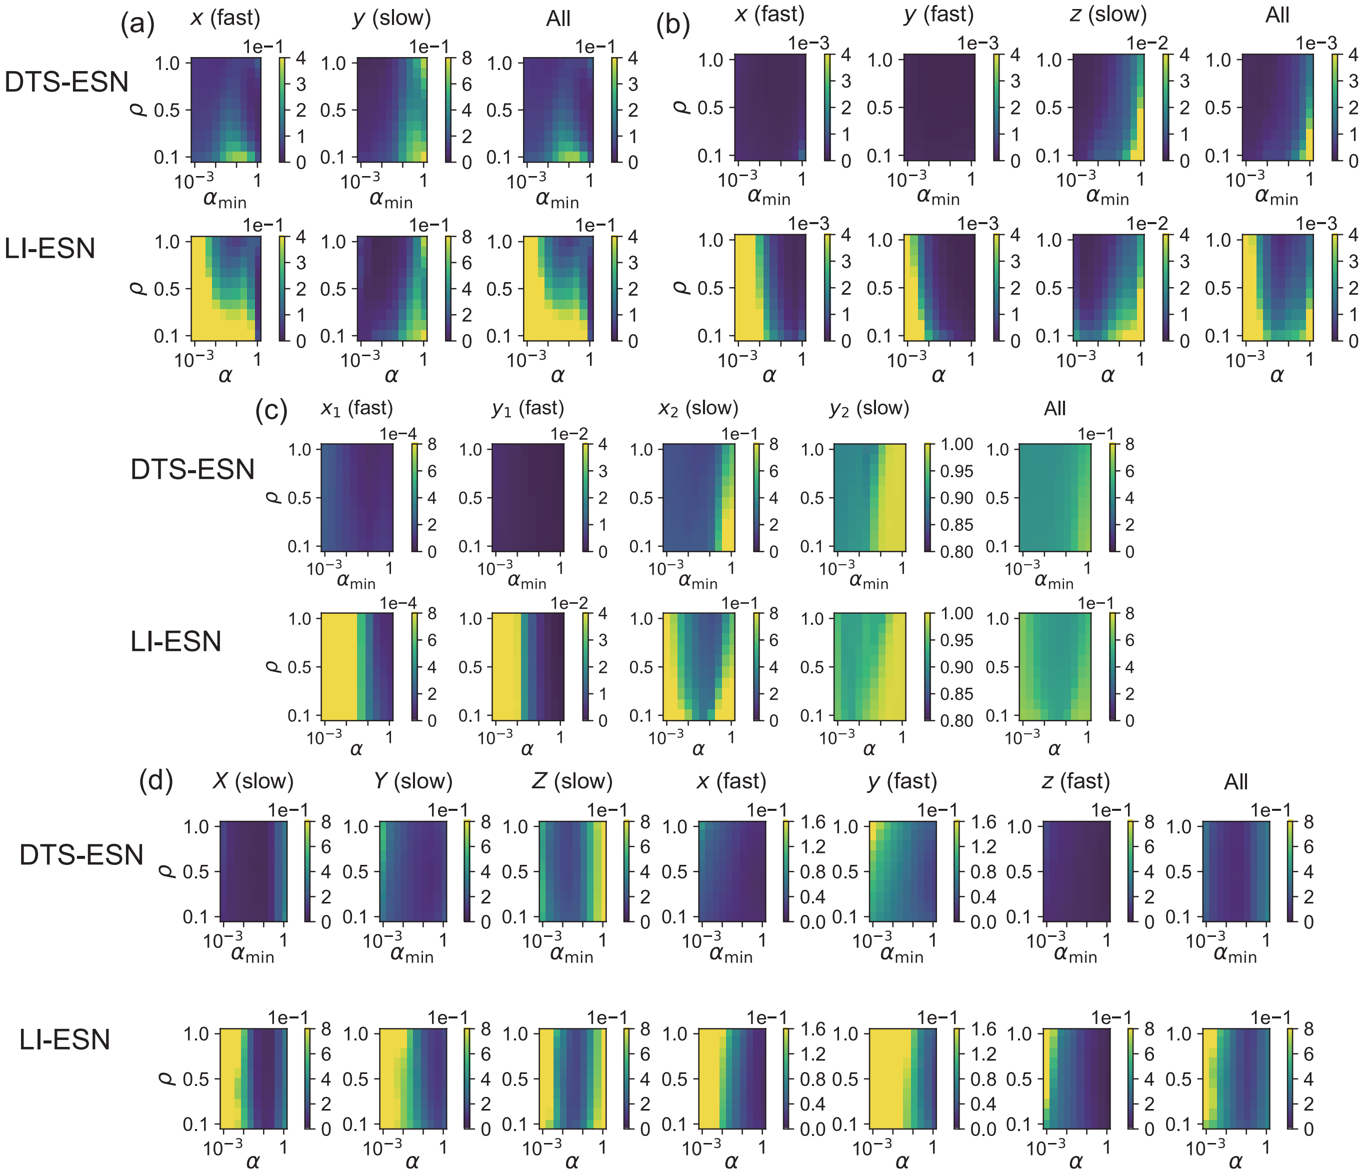


FIG. S6. The effect of the spectral radius $\rho$ on the prediction performance of the DTS-ESN (upper panels) and the LI-ESN (lower panels) in Task 1. The color bar indicates the NRMSE. The horizontal axis is $\alpha_{\rm min}$ for the DTS-ESN and $\alpha$ for the LI-ESN. The hyperparameter and data settings are the same as those for Fig. 3 of the main text, except for the varied ones. (a) The Rulkov model. (b) The Hindmarsh-Rose model. (c) The tc-VdP model. (d) The tc-Lorenz model.

## IV. AUTOREGRESSIVE PREDICTION (TASK 2)

### IV-A. Hyperparameter dependence

Figure 6 in the main text shows the valid time obtained by the closed-loop RC models in the autoregressive prediction task (Task 2). In this figure, we fixed the hyperparameter values other than the leak rates. To validate the result further, we examined the effect of the input scaling factor $\gamma$ on the valid time as shown in Fig. S7 and that of the spectral radius $\rho$ as shown in Fig. S8. The yellow color corresponds to a large valid time, meaning a longer-term successful prediction. For the Rulkov and HR models in Figs. S7(a) and (b), it is clearly seen that the DTS-ESN has more yellow parameter regions compared to the LI-ESN. For the tc-VdP model and the tc-Lorenz model in Figs. S7(c) and (d), there is no clear difference in the size of the yellow regions between the DTS-ESN and the LI-ESN.

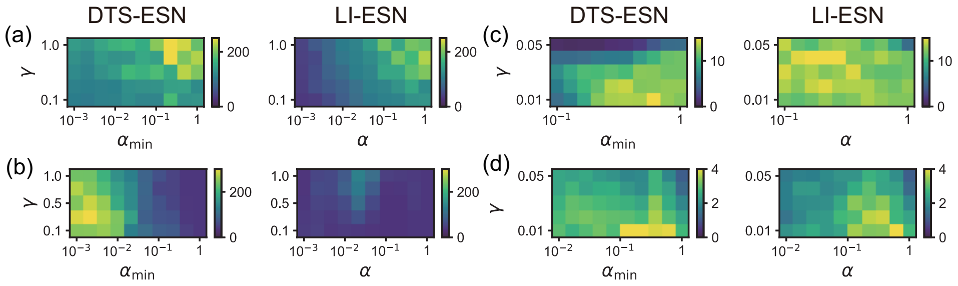


FIG. S7. The effect of the input scaling factor $\gamma$ on the prediction performance of the DTS-ESN (upper panels) and the LI-ESN (lower panels) in Task 2. The color bar indicates the valid time. The horizontal axis is $\alpha_{\min}$ for the DTS-ESN and $\alpha$ for the LI-ESN. The hyperparameter and data settings are the same as those for Fig. 5 of the main text, except for the varied ones. (a) The Rulkov model. (b) The Hindmarsh-Rose model. (c) The tc-VdP model. (d) The tc-Lorenz model.

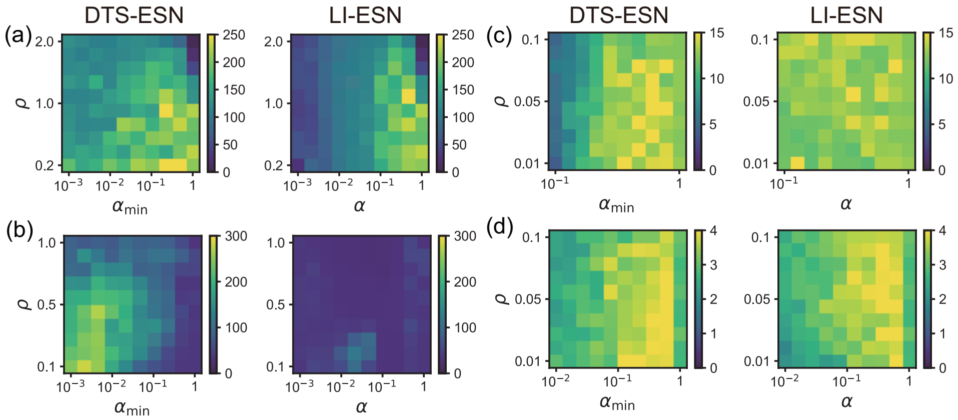


FIG. S8. The effect of the spectral radius $\rho$ on the prediction performance of the DTS-ESN (upper panels) and the LI-ESN (lower panels) in Task 2. The color bar indicates the valid time. The horizontal axis is $\alpha_{\min}$ for the DTS-ESN and $\alpha$ for the LI-ESN. The hyperparameter and data settings are the same as those for Fig. 5 of the main text, except for the varied ones. (a) The Rulkov model. (b) The Hindmarsh-Rose model. (c) The tc-VdP model. (d) The tc-Lorenz model.

### IV-B. Output weight matrix

In Task 2, the input time series are generated from both fast and slow subsystems. Therefore, the reservoir driven by these inputs have both fast and slow timescales even if the leak rate is identical for all the reservoir neurons as in the LI-ESN. When the leak rates are distributed as in the DTS-ESN, there are interactions between the fast/slow responsiveness of the reservoir neurons and the fast/slow inputs. It is a future issue to reveal the mechanism of these interactions. Figure S9 shows the absolute output weights of $\hat{W}^{\rm out}$ of the trained DTS-ESN, plotted against the leak

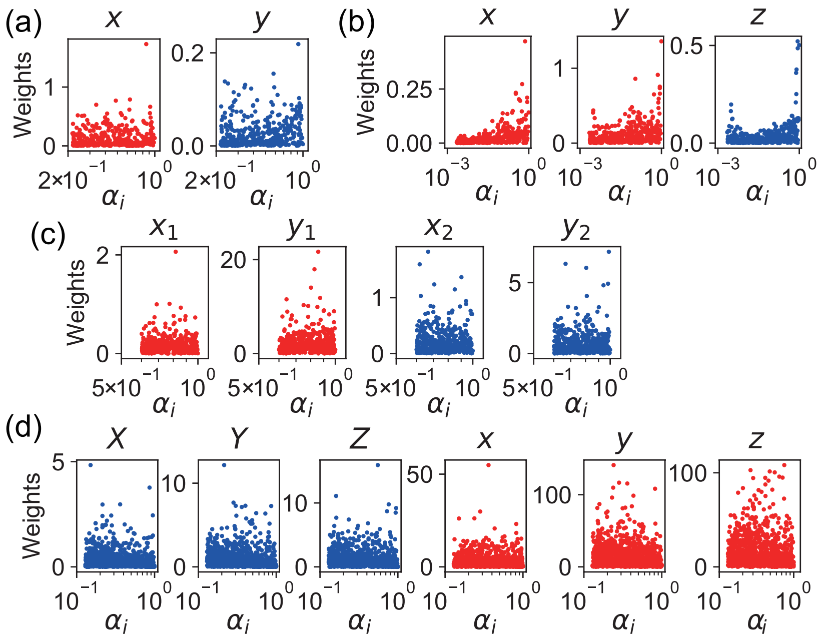


FIG. S9. The absolute output weights in $\hat{W}^{\text{out}}$ of trained DTS-ESN, plotted against the leak rates of the corresponding reservoir neurons. Each panel corresponds to each component of the target system. The parameter values are the same as those for Fig. 5. (a) The Rulkov model. (b) The HR model. (c) The tc-VdP model. (d) The tc-Lorenz model.

rate of the corresponding reservoir neuron. Compared to the counterpart for Task 1 as shown in Fig. 4 of the main text, the plots have no remarkable features.

### IV-C. Lyapunov exponents

The valid time is one of the useful measures for evaluating the long-term prediction ability of the closed-loop RC models. However, the valid time is highly variable depending on the hyperparameter setting and the initial condition at the start of the autoregressive prediction [3]. Another measure for evaluating how well a closed-loop RC model replicates the target dynamical system is the Lyapunov exponent which characterizes the rate of separation of infinitesimally close trajectories of a dynamical system [4, 5]. A set of Lyapunov exponents regarding different orientations of initial separation is called a Lyapunov spectrum. There are positive Lyapunov exponents if the trajectory exhibits chaotic behavior. We numerically estimate the Lyapunov exponents of the trained DTS-ESN and compare them with the actual values computed from the target dynamical system.

We describe how to compute Lyapunov exponents for a closed-loop DTS-ESN which is written as follows (see Eqs. (1)-(3) in the main text):

$$\mathbf{x}(t+\Delta t) = (I-A)\mathbf{x}(t) + A\tanh(((\gamma W^{\text{in}} + \zeta W^{\text{fb}})\hat{W}^{\text{out}} + \rho W)\mathbf{x}(t)), \tag{S15}$$

where $\hat{W}^{\text{out}}$ denotes an optimized output weight matrix. This equation is regarded as an $N_x$-dimensional autonomous discrete-time dynamical system. The Jacobian matrix is given by

$$J(t) = (I-A) + AB \circ (I - \tanh^2(B\mathbf{x}(t))), \tag{S16}$$

where $X \circ Y$ represents the Hadamard product and $B \equiv ((\gamma W^{\text{in}} + \zeta W^{\text{fb}})\hat{W}^{\text{out}} + \rho W)$. We compute the time evolution of the state vector $\mathbf{x}(t)$ of the closed-loop model and evaluate the Jacobian matrix $J(t)$ at each time. We used the QR decomposition method for the computation [6]. We denote by $e_i$ the eigenvalues of

$$L = (M^\top(t)M(t))^{1/2t}, \tag{S17}$$

where $M = J(t-\Delta t)J(t-2\Delta t)\cdots J(0)$. The Lyapunov exponents are obtained as follows:

$$l_i = \frac{\ln e_i}{t/\Delta t} \quad \text{for } i = 1, \ldots, N_x. \tag{S18}$$

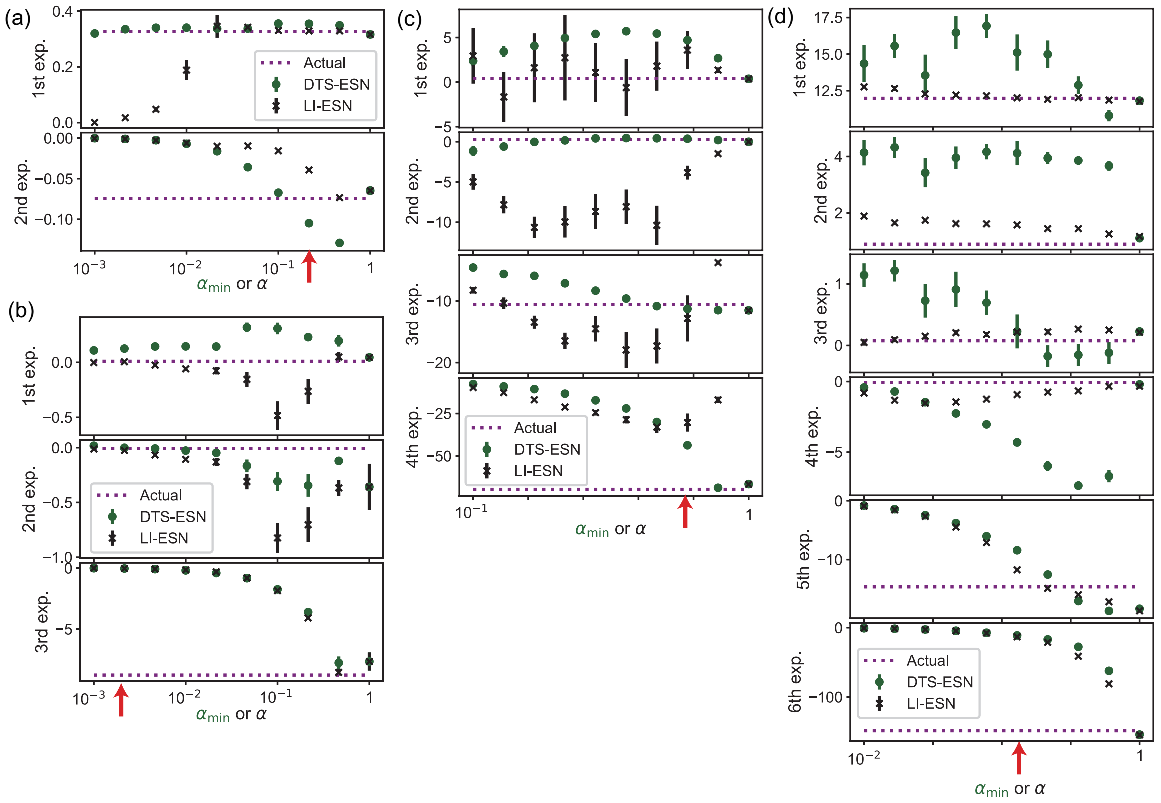


FIG. S10. Largest Lyapunov exponents of the DTS-ESN plotted against $\alpha_{\rm min}$ and those of the LI-ESN plotted against $\alpha$. The hyperparameter and data settings are the same as those for Fig. 6 in the main text. The red arrows indicate the $\alpha_{\rm min}$ values at which the largest average valid time was obtained. The actual Lyapunov exponents of the target dynamical systems are plotted as a reference. (a) The Rulkov model. (b) The HR model. (c) The tc-VdP model. (d) The tc-Lorenz model.

The Lyapunov exponents are sorted in descending order.

Figure S10 shows the Lyapunov exponents for the DTS-ESN (green circles), those for the LI-ESN (black crosses), and the actual values for the target systems (purple dotted lines). The hyperparameter values are the same as those used for Fig. 6 in the main text. The red arrows indicate the leak rate values corresponding to the largest valid time obtained by the DTS-ESN in Fig. 6. In Fig. S10(a), the two largest Lyapunov exponents of the DTS-ESN are close to the actual values at the condition where the valid time is largest. However, in the other cases, a closeness of the estimated Lyapunov exponents to the actual values seems not to necessarily correspond to the largest valid time. It is a future work to clarify the relationship between the nonlinear characteristics of the chaotic behavior produced by the closed-loop DTS-ESN and its prediction ability.


[1] H. Jaeger, M. Lukoševičius, D. Popovici, and U. Siewert, Optimization and applications of echo state networks with leaky-integrator neurons, Neural Networks **20**, 335 (2007).

[2] L. Manneschi, M. O. Ellis, G. Gigante, A. C. Lin, P. Del Giudice, and E. Vasilaki, Exploiting multiple timescales in hierarchical echo state networks, Frontiers in Applied Mathematics and Statistics **6**, 76 (2021).

[3] J. Pathak, A. Wikner, R. Fussell, S. Chandra, B. R. Hunt, M. Girvan, and E. Ott, Hybrid forecasting of chaotic processes: Using machine learning in conjunction with a knowledge-based model, Chaos: An Interdisciplinary Journal of Nonlinear Science **28**, 041101 (2018).

[4] J. Pathak, Z. Lu, B. R. Hunt, M. Girvan, and E. Ott, Using machine learning to replicate chaotic attractors and calculate lyapunov exponents from data, Chaos: An Interdisciplinary Journal of Nonlinear Science **27**, 121102 (2017).

[5] T. Akiyama and G. Tanaka, Analysis on characteristics of multi-step learning echo state networks for nonlinear time series prediction, in *2019 International Joint Conference on Neural Networks (IJCNN)* (IEEE, 2019) pp. 1–8.

[6] K. Geist, U. Parlitz, and W. Lauterborn, Comparison of different methods for computing lyapunov exponents, Progress of theoretical physics **83**, 875 (1990).
